# Supplementary material for: Similarity Problems in High Dimensions
Source: arXiv:1906.04842 source file (2019-06-11)
Supplement: Supplementary file 1 [file appendix.tex]

\appendix
\section{Binomial and Hamming ball volume bounds}\label{appendix:A}

\begin{lemma}[Binomial bounds] 
Let $1 \leq k \leq n = \omega(1)$. Then:

\begin{enumerate}
\item If $k = O(1)$, ${n \choose k} = (1+o(1))n^k/k!$.
\item If $k = \omega(1)$ and $k = o(\sqrt{n})$, 
\[ {n \choose k} = (1+o(1)) \frac{1}{\sqrt{2 \pi k}} \left( \frac{ne}{k} \right)^{k}. \]
\item If $k = o(n)$, $\log {n \choose k} = (1+o(1))k \log (n/k)$.
\item If $k  = \Omega(n)$, $\log {n \choose k} = (1+o(1)) H(k/n)n$, where $H(p) = -p \log p - (1-p) \log (1-p)$ is the binary entropy function defined on $[0,1]$.
\end{enumerate}
\end{lemma}

Next, recall that $\B[d]{}{R}$ denotes the volume of a Hamming ball of radius $R$ in $d$-dimensions.
\begin{lemma}\label{hammingbounds}[Hamming ball bounds] Assume that $R \leq d/2$. The following are upper bounds on $|B_{d}(R)|$:
\begin{enumerate}
\item (Trivial)  $\forall R \leq d/2, \ \B[d]{}{R}\leq R {d \choose R}$.
\item (Small $R$) When $R= o(\sqrt{d})$,  $\B[d]{}{R} \leq 2 {d \choose R}$.
\item (Large R) Let $D(x||y) = x \log (x/y) + (1-x) \log ((1-x)/(1-y))$ denote the ``relative entropy'' or Kullback-Leibler Divergence\footnote{Note that $D(p||1/2) = 1-H(p)$.
}, defined for $0 \leq x,y \leq 1$. Then

\[ \frac{2^d}{\sqrt{2 \pi d}} exp(-d D(R/d||1/2)) \leq  \B[d]{}{R} \leq 2^d exp(-d D(R/d||1/2)).\]

\end{enumerate}
\end{lemma}

%%% Local Variables:
%%% mode: latex
%%% TeX-master: "main"
%%% End:
